# Supplementary material for: SAT-based Formal Fault-Resistance Verification of Cryptographic Circuits
Source: arXiv:2307.00561 source file (2023-07-02)
Supplement: Supplementary file 1 [file appendix-2.tex]

\section{Fault Type Reduction}
In this subsection, we propose a novel technique to reduce the set of fault types $\{ \tau_{s},\tau_{r},\tau_{bf}\}$ to the bit-flip one $\tau_{bf}$,
thus, reduce the size of the resulting Boolean formulas and improve the efficiency of fault-resistance verification.

The fault type reduction is inspired by the following observation.
Consider a fault event $\EE(\alpha,\beta,\tau)$ with $\tau\in \mathcal{T}=\{ \tau_{s},\tau_{r},\tau_{bf}\}$. For any fixed sequence of primary inputs $(\vec{x}_{1},\cdots,\vec{x}_{k})$,
either the output signal of the gate $\beta$ does not change or changes.
If the output signal of the gate $\beta$ does not change, then the fault event $\EE(\alpha,\beta,\tau)$ will not affect
the primary outputs. If the output signal of the gate $\beta$ changes, it is flipped either from
$\Gone$ to $\Gzero$ or from $\Gzero$ to $\Gone$,  the same effect can be achieved by applying
the fault event $\EE(\alpha,\beta,\tau_{bf})$. Thus, the fault type $\tau_{bf}$ is sufficient
for verifying whether the circuit $\SeqC'$ is fault resistant or not even all the fault types $\{ \tau_{s},\tau_{r},\tau_{bf}\}$ are considered.
%This observation yields the following theorem.

\begin{theorem} \label{thm:faulttypereduce}
Given a fault-resistance model $\zeta(\Nn_e,\Nn_c,\mathcal{T},\ell)$ for $\SeqC'$ and a fault vector $\VV(\SeqC',\BB)\in \sem{\zeta(\Nn_e,\Nn_c,\mathcal{T},\ell)}$,
let $\VV_{bf}(\SeqC',\BB)$ be the fault vector $\{\EE(\alpha,\beta,\tau_{bf})\mid \EE(\alpha,\beta,\tau)\in \VV(\SeqC',\BB)\}$.
If the fault vector $\VV(\SeqC',\BB)$ is effective on the circuit $\SeqC'$,
then there exists a fault vector $\VV'(\SeqC',\BB)\subseteq \VV_{bf}(\SeqC',\BB)$
that is also effective on the circuit $\SeqC'$.

Moreover, if $|\VV(\SeqC',\BB)|=1$, then $\VV_{bf}(\SeqC',\BB)$
is an effective fault vector on the circuit $\SeqC'$.
\end{theorem}
\begin{proof}
Suppose the fault vector $\VV(\SeqC',\BB)$ is effective on the circuit $\SeqC'$.
Let us apply induction on the number $n$ of fault events $\EE(\alpha,\beta,\tau)\in \VV(\SeqC',\BB)$ such that
$\tau\neq \tau_{bf}$. The result immediately follows if $n=0$, as $\VV(\SeqC',\BB)=\VV_{bf}(\SeqC',\BB)$.

Suppose $n\geq 1$. Consider a fault event $\EE(\alpha,\beta,\tau) \in \VV(\SeqC',\BB)$ such that $\tau\neq \tau_{bf}$.
We define the following two fault vectors:
\begin{center}
$\VV^1(\SeqC',\BB)=\VV(\SeqC',\BB)\setminus \{\EE(\alpha,\beta,\tau)\}$ and
   $\VV^2(\SeqC',\BB)=\VV^1(\SeqC',\BB)\cup \{\EE(\alpha,\beta,\tau_{bf})\}$.
\end{center}

Since $\VV(\SeqC',\BB)$ is effective on the circuit $\SeqC'$,
there exists a sequence of primary inputs $(\vec{x}_{1},\cdots,\vec{x}_{k})$ such that
the sequences of primary outputs $\sem{\SeqC'}(\vec{x}_1,\cdots, \vec{x}_k)$
and $\sem{\SeqC'[\VV(\SeqC',\BB)]}(\vec{x}_1,\cdots, \vec{x}_k)$ differ at
some clock cycle before the error flag output $o_{\tt flag}$ differs.
We proceed by distinguishing whether the output signal of the gate $\beta$ differs in the circuits
$\SeqC'$ and $\SeqC'[\VV(\SeqC',\BB)]$ under the same sequence of primary inputs $(\vec{x}_{1},\cdots,\vec{x}_{k})$.

\begin{itemize}
\item  If the output signal of the gate $\beta$ is the same in the circuits
$\SeqC'$ and $\SeqC'[\VV(\SeqC',\BB)]$ under the same sequence of primary inputs $(\vec{x}_{1},\cdots,\vec{x}_{k})$,
then the fault event $\EE(\alpha,\beta,\tau)$ does not affect the output signal of the gate $\beta$.
It implies that the sequences of primary outputs $\sem{\SeqC'[\VV(\SeqC',\BB)]}(\vec{x}_1,\cdots, \vec{x}_k)$ and
$\sem{\SeqC'[\VV^1(\SeqC',\BB)]}(\vec{x}_1,\cdots, \vec{x}_k)$ are the same.
Thus, $\VV^1(\SeqC',\BB)$ is an effective fault vector on the circuit $\SeqC'$.
By applying the induction hypothesis, $\VV^1_{bf}(\SeqC',\BB)$ is an effective fault vector on the circuit $\SeqC'$.
The result immediately follows from the fact that $\VV^1_{bf}(\SeqC',\BB) \subset \VV_{bf}(\SeqC',\BB)$.

\item  If the output signal of the gate $\beta$ differs in the circuits
$\SeqC'$ and $\SeqC'[\VV(\SeqC',\BB)]$ under the same sequence of primary inputs $(\vec{x}_{1},\cdots,\vec{x}_{k})$,
then the fault event $\EE(\alpha,\beta,\tau)$ flips the output signal of the gate $\beta$.
It implies that the sequences of primary outputs $\sem{\SeqC'[\VV(\SeqC',\BB)]}(\vec{x}_1,\cdots, \vec{x}_k)$ and
$\sem{\SeqC'[\VV^2(\SeqC',\BB)]}(\vec{x}_1,\cdots, \vec{x}_k)$ are the same. Thus, $\VV^2(\SeqC',\BB)$ is an effective fault vector on the circuit $\SeqC'$.
By applying the induction hypothesis, $\VV^2_{bf}(\SeqC',\BB)$ is an effective fault vector on the circuit $\SeqC'$.
The result immediately follows from the fact that $\VV^2_{bf}(\SeqC',\BB)\subseteq \VV_{bf}(\SeqC',\BB)$.
\end{itemize}

Moreover, if $|\VV(\SeqC',\BB)|=1$, then the output signal of the gate $\beta$ must differ in the circuits
$\SeqC'$ and $\SeqC'[\VV(\SeqC',\BB)]$ under the same sequence of primary inputs $(\vec{x}_{1},\cdots,\vec{x}_{k})$,
otherwise $\VV(\SeqC',\BB)$ is not an effective fault vector on the circuit $\SeqC'$.
Thus, $\VV^2_{bf}(\SeqC',\BB)=\VV_{bf}(\SeqC',\BB)$
is an effective fault vector on the circuit $\SeqC'$.
\end{proof}

By applying Theorem~\ref{thm:faulttypereduce}, to verify whether $\langle\SeqC',\BB\rangle\models \zeta(\Nn_e,\Nn_c,T,\ell)$
for any $T\subseteq \mathcal{T}$, it suffice to verify whether $\langle\SeqC',\BB\rangle\models \zeta(\Nn_e,\Nn_c,\{\tau_{bf}\},\ell)$ holds or not.

\begin{corollary}\label{cor:faulttypereduce}
If $\langle\SeqC',\BB\rangle\models \zeta(\Nn_e,\Nn_c,\{\tau_{bf}\},\ell)$, then $\langle\SeqC',\BB\rangle\models \zeta(\Nn_e,\Nn_c,\mathcal{T},\ell)$.
\end{corollary}

\begin{example} \label{emp:SATencodingwithfaulttypereduce}
Recall that the fault-resistance verification problem of the illustrating example w.r.t the fault-resistance model $\zeta(1,1,\mathcal{T},\Cc)$
and the blacklist $\BB$ is reduced to SAT solving of
the Boolean formula $\Psi_{fr}$ in Example~\ref{emp:SATencoding},
where $\Psi_{fr}=  \Psi_{\Nn_c}\wedge \Psi_{\Nn_e}\wedge \big(\bigvee_{o\in\{\tt w,x,y,z\}}\psi_{1,o}\neq \psi_{1,o}''\big) \wedge \neg\psi_{1,{\tt flag}}''\bigwedge_{i=1}^{12} \phi_{i}$.
By Corollary~\ref{cor:faulttypereduce}, it suffices to consider
$T=\{\tau_{bf}\}$. Thus,
the gadgets of the form $G_{\bullet,\mathcal{T}}(in_1,in_2,c,b_1,b_2)$ and $G_{\bullet,\mathcal{T}}(in,c,b_1,b_2)$ in $\Psi_{fr}$ could be replaced by
 the gadgets $G_{\bullet,T}(in_1,in_2,c)$ and $G_{\bullet,\mathcal{T}}(in,c)$, respectively.
For instance, $\phi_1:=g_1\Leftrightarrow G_{\oplus,\mathcal{T}}''(b,c,c_1,b_{1,1},b_{1,2})$
is simplified to $\phi_1':=g_1\Leftrightarrow G_{\oplus,T}''(b,c,c_1)$.
It eliminates the Boolean variables of selection inputs ($b,b_1,b_2$) and reduces the number of clauses.
We denote by $\Psi_{fr}'=  \Psi_{\Nn_c}\wedge \Psi_{\Nn_e}\wedge \big(\bigvee_{o\in\{\tt w,x,y,z\}}\psi_{1,o}\neq \psi_{1,o}''\big) \wedge \neg\psi_{1,{\tt flag}}''\bigwedge_{i=1}^{12} \phi_{i}'$
the simplified Boolean formula.
\end{example}

\section{More Aggressive Vulnerable Gate Reduction}
The more aggressive vulnerable gate reduction is inspired by the following observation.
Consider a sub-circuit $S$ of the circuit $\SeqC'$ in the $\alpha$-th clock cycle such that the output signal of the sub-circuit $S$
is the output of a logic gate $\beta$.
For any fixed fault vector $\VV(\SeqC',\BB)$ to the sub-circuit $S$ with fault type $\tau_{bf}$
and any fixed sequence of primary inputs $(\vec{x}_{1},\cdots,\vec{x}_{k})$,
the output signal of the gate $\beta$ either changes or does not change.
If the output signal of the gate $\beta$ does not change,
then the effect of the fault vector $\VV(\SeqC',\BB)$ is stopped by the gate $\beta$ and will not
affect the primary outputs. If the output signal of the gate $\beta$ changes,
it is flipped either from $\Gone$ to $\Gzero$ or from $\Gzero$ to $\Gone$, the same effect can be achieved by applying
only one fault event $\EE(\alpha,\beta,\tau_{bf})$.
Thus, it suffices to consider fault injections on the gate $\beta$ instead of the other gates of the sub-circuit $S$ if $\beta\not\in\BB$,
consequently, reduces the number of considered gates when verifying fault resistance.

Formally, a sub-circuit $S$ is called \emph{single-exit sub-circuit}, more specifically, \emph{$\beta$-exit sub-circuit}, in the circuit $\SeqC'$, if its unique output is output of the logic gate $\beta$ and it only contains gates
in the same $\alpha$-th clock cycle as the gate $\beta$.
A single-exit sub-circuit $S$ is \emph{maximal} if no other single-exit sub-circuit $S'$ exists %for any logic gate $\beta'\not\in \BB$ in the circuit $\SeqC'$
such that $S$ is a proper sub-circuit of $S'$.

Let $\VV(\SeqC',\BB)=\VV_1(\SeqC',\BB)\cup \VV_2(\SeqC',\BB)\in \sem{\zeta(\Nn_e,\Nn_c,\{\tau_{bf}\},\ell)}$ be an effective fault vector on the circuit $\SeqC'$
such that $\VV_2(\SeqC',\BB)$ is a fault vector on the $\beta$-exit sub-circuit $S$,
namely, i.e., it only contains fault events $\EE(\alpha,\beta',\tau_{bf})$ for $\beta'\in R_{\alpha-1}'\cup V_\alpha'\setminus (I'_\alpha\cup O'_\alpha)$.
Let $\VV'(\SeqC',\BB)=\VV_1(\SeqC',\BB)\cup \{\EE(\alpha,\beta,\tau_{bf})\}$.
We have:

 \begin{theorem} \label{thm:aggfaultgatereduce}
If $\beta\not\in\BB$ and $\ell\in\{\Cc,\CR\}$, % such that $a'$ is a logic gate (resp. memory gate) if $\ell=\Cc$ (resp. $\ell=\Rr$).
then $\VV'(\SeqC',\BB)\in \sem{\zeta(\Nn_e,\Nn_c,\{\tau_{bf}\},\ell)}$
and there exists a fault vector $\VV''(\SeqC',\BB)\subseteq \VV'(\SeqC',\BB)$
that is effective on the circuit $\SeqC'$.

Moreover, if $\VV_1(\SeqC',\BB)=\emptyset$, then $\{\EE(\alpha,\beta,\tau_{bf})\}$ is an effective fault vector on the circuit $\SeqC'$.
\end{theorem}

\begin{proof}
Following from the facts that $\beta$ is a logic gate, $\beta\not\in\BB$ and $\ell\in\{\Cc,\CR\}$,
it is easy to see that $\VV'(\SeqC',\BB)\in \sem{\zeta(\Nn_e,\Nn_c,\{\tau_{bf}\},\ell)}$.

Since $\VV(\SeqC',\BB)$ is an effective fault vector on the circuit $\SeqC'$,
there exists a sequence of primary inputs $(\vec{x}_{1},\cdots,\vec{x}_{k})$ such that
 $\sem{\SeqC'}(\vec{x}_1,\cdots, \vec{x}_k)$
and $\sem{\SeqC'[\VV(\SeqC',\BB)]}(\vec{x}_1,\cdots, \vec{x}_k)$ differ at
some clock cycle before the error flag output $o_{\tt flag}$ differs.
We proceed by distinguishing whether the output signal of the gate $\beta$ differs in the circuits
$\SeqC'$ and $\SeqC'[\VV(\SeqC',\BB)]$ under the same sequence of primary inputs $(\vec{x}_{1},\cdots,\vec{x}_{k})$.

\begin{itemize}
  \item If the output signal of the gate $\beta$ is the same in the circuits
$\SeqC'$ and $\SeqC'[\VV(\SeqC',\BB)]$ under the same sequence of primary inputs $(\vec{x}_{1},\cdots,\vec{x}_{k})$,
then the effects of the fault events of $\VV_2(\SeqC',\BB)$ are stopped at the gate $\beta$, as
the output of the $\beta$-exit sub-circuit $S$ is the output of the gate $\beta$. Thus,
$\sem{\SeqC'[\VV(\SeqC',\BB)]}(\vec{x}_1,\cdots, \vec{x}_k)$
and $\sem{\SeqC'[\VV_1(\SeqC',\BB)]}(\vec{x}_1,\cdots, \vec{x}_k)$ are the same.
It implies that  $\sem{\SeqC'}(\vec{x}_1,\cdots, \vec{x}_k)$
and $\sem{\SeqC'[\VV_1(\SeqC',\BB)]}(\vec{x}_1,\cdots, \vec{x}_k)$ differ at
some clock cycle before the error flag output $o_{\tt flag}$ differs.
The result immediately follows.

\item If the output signal of the gate $\beta$ differs in the circuits
$\SeqC'$ and $\SeqC'[\VV(\SeqC',\BB)]$ under the same sequence of primary inputs $(\vec{x}_{1},\cdots,\vec{x}_{k})$,
then the fault propagation from fault events of $\VV_2(\SeqC',\BB)$ flips the output signal of the gate $\beta$.
It implies that  $\sem{\SeqC'[\VV(\SeqC',\BB)]}(\vec{x}_1,\cdots, \vec{x}_k)$
and $\sem{\SeqC'[\VV'(\SeqC',\BB)]}(\vec{x}_1,\cdots, \vec{x}_k)$ are the same, as
the output of the $\beta$-exit sub-circuit $S$ is the output of the gate $\beta$.
Thus,  $\sem{\SeqC'}(\vec{x}_1,\cdots, \vec{x}_k)$
and $\sem{\SeqC'[\VV'(\SeqC',\BB)]}(\vec{x}_1,\cdots, \vec{x}_k)$ differ at
some clock cycle before the error flag output $o_{\tt flag}$ differs. The result immediately follows.
\end{itemize}

Moreover, if $\VV_1(\SeqC',\BB)=\emptyset$, then the output signal of the gate $\beta$ must differ in the circuits
$\SeqC'$ and $\SeqC'[\VV(\SeqC',\BB)]$ under the same sequence of primary inputs $(\vec{x}_{1},\cdots,\vec{x}_{k})$,
otherwise $\VV(\SeqC',\BB)$ is ineffective on the circuit $\SeqC'$.
The result follows from the fact that $\VV'(\SeqC',\BB)=\{\EE(\alpha,\beta,\tau_{bf})\}$.
\end{proof}

Now, the problem is how to efficiently identify maximal single-exit sub-circuits in the circuit $\SeqC'$  so that
the number of fault events that should be considered is minimized when verifying fault-resistance. To solve this problem,
we propose a graph traversal based algorithm, i.e., Algorithm~\ref{alg:sub-circuits}, which
 returns a set of maximal single-exit sub-circuits  for a given $k$-clock cycle circuit $\SeqC'$ and a blacklist $\BB$.

In detail, Algorithm~\ref{alg:sub-circuits} first initializes two empty maps: $M_1$ from gates to gates and $M_2$ from gates to sets of gates (Line~\ref{alg:sub-circuits:init}).
For each gate $\beta$, if $M_1[\beta]$ is the gate $\beta'$, then the gate $\beta$ is included
in the $\beta'$-exit sub-circuit, and $M_2[\beta']$ is the set of gates that are included in the $\beta'$-exit sub-circuit.
We remark that $M_2[\beta']$ will be the singleton set $\{\beta'\}$ if $\beta'$ is connected to some registers, and no gates
except for $\beta'$ can be added into the set $M_2[\beta']$ if $\beta'\in\BB$ or $\beta'\in\RR$.
Next, for each clock cycle $i\in [k]$, the outer-loop (Lines~\ref{alg:sub-circuits:loop1start}--\ref{alg:sub-circuits:loop1end})
computes maximal single-exit sub-circuits of $\SeqC'$ in the $i$-th clock cycle.

During the $i$-th iteration of the outer-loop, Algorithm~\ref{alg:sub-circuits} iteratively traverses each gate $\beta$ of $R_{i-1}\cup V_i'\setminus (I_i'\cup O'_i)$ in a
reverse topological sort (Lines~\ref{alg:sub-circuits:loop2start}--\ref{alg:sub-circuits:loop2end}).
For each gate $\beta\in R_{i-1}\cup V_i'\setminus (I_i'\cup O'_i)$,
if all the successors $\{\beta_1,\cdots, \beta_m\}$ of $\beta$ are included in the $\beta'$-exit sub-circuit for some logic gate $\beta'$ (i.e., $M_1[\beta_1]=M_1[\beta_2]=\cdots=M_1[\beta_m]=\beta'$)
and the gate $\beta'$ is vulnerable (i.e., $\beta'\not\in\BB$),
then $\beta$ is added into the  $\beta'$-exit sub-circuit by updating the maps $M_1$ and $M_2$ accordingly (Lines~\ref{alg:sub-circuits:if1}--\ref{alg:sub-circuits:if2}).
Otherwise, $\beta$ is added into the set $M_2[\beta]$, forming the $\beta$-exit sub-circuit, where
$M_1$ is updated accordingly (Lines~\ref{alg:sub-circuits:else1}--\ref{alg:sub-circuits:else2}).

Finally, Algorithm~\ref{alg:sub-circuits} returns the map $M_2$ such that
for each logic gate $\beta\not\in \BB$, $M_2[\beta]$ forms the maximal $\beta$-exit sub-circuit. Furthermore,
it is well-known that a topological sort of a DAG can be computed in
linear time of the number of vertices and edges, thus the map $M_2$ can be computed in linear time of the number of vertices and edges of $\SeqC'$.

\begin{lemma}
Algorithm~\ref{alg:sub-circuits} is in linear time of the number of vertices and edges of $\SeqC'$
and for each logic gate $\beta\not\in \BB$, $M_2[\beta]$ forms the maximal $\beta$-exit sub-circuit.
\end{lemma}

By Theorem~\ref{thm:aggfaultgatereduce},
only the fault events on the gates $\beta$ such that $M_2[\beta]$ is defined and $\beta\not\in\BB$ should be considered.
Let $\BB'$ be the set of gates $\beta$ such that $M_2[\beta]$ is undefined.
We have:

\begin{corollary}\label{cor:aggfaultgatereduce}
If $\langle\SeqC',\BB\cup\BB'\rangle\models \zeta(\Nn_e,\Nn_c,\{\tau_{bf}\},\ell)$
and $\ell\in\{\Cc, \CR\}$, then $\langle\SeqC',\BB\rangle\models \zeta(\Nn_e,\Nn_c,\{\tau_{bf}\},\ell)$.
\end{corollary}

%some successors of $\beta$ are included in more than one single-exit sub-circuit or
%are included in the blacklist $\BB'$ or are registers.

\begin{algorithm}[t]
\SetAlgoLined
\caption{Identifying maximal single-exit sub-circuits}
\label{alg:sub-circuits}
\KwIn{A $k$-clock cycle circuit $\SeqC'=(\II,\OO',\RR', \vec{s}_0', \CC')$, where $\RR'=R_0'\uplus \cdots \uplus R_k'$, $\CC'=\{C_1',\cdots, C_k'\}$, $C_i'=(V_i',I_i', O_i', E_i',\gate_i')$ for each $i\in[k]$ and a blacklist $\BB$}
\KwOut{A set of maximal single-exit sub-circuits of $\SeqC'$}
    Let $M_1$ and $M_2$ be two empty maps from gates to gates and sets of gates, respectively\; \label{alg:sub-circuits:init}
    \ForEach{$i\in[k]$}
    {  \label{alg:sub-circuits:loop1start}
        Let $Q$ be the list of gates of $R_{i-1}\cup V_i'\setminus (I_i'\cup O'_i)$ in a reverse topological sort\;
        \ForEach{$\beta\in Q$}{   \label{alg:sub-circuits:loop2start}
            Let $\{\beta_1,\cdots, \beta_m\}$ be the successors of $\beta$ including gates and primary outputs\;  \label{alg:sub-circuits:successors}
            \If{$M_1[\beta_1]=M_1[\beta_2]=\cdots=M_1[\beta_m]=\beta'\wedge \beta'\not\in \BB\wedge \beta'\in V_i'\setminus (I_i'\cup O'_i)$}
            {
                Add $\beta$ into the set $M_2[\beta']$\;   \label{alg:sub-circuits:if1}
                $M_1[\beta]\gets \beta'$\;  \label{alg:sub-circuits:if2}
            }
            \Else{
                Add $\beta$ into the set $M_2[\beta]$\;    \label{alg:sub-circuits:else1}
                $M_1[\beta]\gets \beta$\;    \label{alg:sub-circuits:else2}
            } \label{alg:sub-circuits:loop2end}
        }  \label{alg:sub-circuits:loop1end}
  }
  \Return{$M_2$\;}
\end{algorithm}

\begin{example} \label{emp:SATencodingwithgatereduce}
Consider the illustrating example.
We have: $M_2[{\tt p6}]=\{{\tt p1,p2,p3,p4,p5,p6}\}$,
$M_2[{\tt s11}]=\{{\tt s_8,s11}\}$, $M_2[{\tt s10}]=\{{\tt s7,s10}\}$,
$M_2[{\tt s9}]=\{{\tt s4,s9}\}$, $M_2[{\tt s6}]=\{{\tt s5,s6}\}$,
and $M_2[\beta]=\{\beta\}$ for any other gate $\beta$.
\end{example}
